# Supplementary material for: PTD-SQL: Partitioning and Targeted Drilling with LLMs in Text-to-SQL
Source: arXiv:2409.14082 source file (2024-09-21)
Supplement: Supplementary file 1 [file appendix.tex]

\onecolumn
\newpage
% Reset depth to add sections and subsections to ToC
\addtocontents{toc}{\protect\setcounter{tocdepth}{3}}

\tableofcontents % Lists only the appendix sections and subsections

\newpage
% %%%%%%%%%%%%%%%%%%%%%%%%%%%%%%%%%%%%%%%%%%%
\section{Statistics of }
\label{appx:statistics}

% %%%%%%%%%%%%%%%%%%%%%%%%%%%%%%%%%%%%%%%%%%%
\newpage
\section{Manual Quality Check}

\subsection{Critique prompt}

\newpage
\subsection{Correction prompt}
